# Supplementary material for: Enhancing Interpretability Through Loss-Defined Classification Objective in Structured Latent Spaces
Source: arXiv:2412.08515 source file (2024-12-11)
Supplement: Supplementary file 1 [file appendix.tex]

\section{Lambda Variation in Preliminary Experiment}
The \Cref{tab:base_1,tab:base_2,tab:base_3} present the complete set of $\lambda$ variations in the range of 0.1 to 0.9 across our weighted sum equation to combine distance and probabilistic loss. 
The results cover the four selected experiments of traditional distance metrics trained on the three setups of models and datasets.

\label{sec:lambda_variation}

\begin{table}[ht]

\centering
\footnotesize
\caption{Baseline comparison with extended $\lambda$ values for Fashion MNIST}
\label{tab:base_1}
\begin{tabular}{ccccc}

\textbf{Dataset} & \textbf{Loss Type} & $\boldsymbol{\lambda}$ & \textbf{Accuracy (Mean ± Std)} & \textbf{Micro-F1 (Mean ± Std)} \\
\hline
\multirow{45}{*}{\textbf{Fashion MNIST}} 
    & Baseline & 0.0  & 88.59 ± 0.15  & 0.8867 ± 0.0020 \\
    \cline{2-5}
    & \multirow{9}{*}{Contrast}& 0.1  & 88.71 ± 0.10  & 0.8870 ± 0.0017 \\
    &                          & 0.2  & 88.78 ± 0.12  & 0.8875 ± 0.0016 \\
    &                          & 0.25 & 88.83 ± 0.08  & 0.8884 ± 0.0015 \\
    &                          & 0.3  & 88.85 ± 0.12  & 0.8887 ± 0.0018 \\
    &                          & 0.4  & 88.90 ± 0.11  & 0.8893 ± 0.0017 \\
    &                          & 0.5  & 88.57 ± 0.14  & 0.8850 ± 0.0019 \\
    &                          & 0.6  & 88.45 ± 0.15  & 0.8842 ± 0.0020 \\
    &                          & 0.7  & 88.33 ± 0.16  & 0.8830 ± 0.0021 \\
    &                          & 0.75 & 87.79 ± 0.25  & 0.8773 ± 0.0022 \\
    &                          & 0.8  & 87.55 ± 0.22  & 0.8749 ± 0.0020 \\
    &                          & 0.9  & 87.30 ± 0.25  & 0.8725 ± 0.0025 \\
\cline{2-5}
    & \multirow{9}{*}{Triplet} & 0.1  & 88.95 ± 0.18  & 0.8890 ± 0.0017 \\
    &                          & 0.2  & 89.05 ± 0.19  & 0.8905 ± 0.0016 \\
    &                          & 0.25 & 89.13 ± 0.18  & 0.8909 ± 0.0011 \\
    &                          & 0.3  & 89.18 ± 0.20  & 0.8911 ± 0.0018 \\
    &                          & 0.4  & 89.23 ± 0.21  & 0.8917 ± 0.0020 \\
    &                          & 0.5  & 89.13 ± 0.34  & 0.8915 ± 0.0036 \\
    &                          & 0.6  & 89.10 ± 0.33  & 0.8909 ± 0.0034 \\
    &                          & 0.7  & 89.05 ± 0.30  & 0.8905 ± 0.0031 \\
    &                          & 0.75 & 88.97 ± 0.33  & 0.8900 ± 0.0038 \\
    &                          & 0.8  & 88.85 ± 0.32  & 0.8887 ± 0.0035 \\
    &                          & 0.9  & 88.73 ± 0.28  & 0.8875 ± 0.0030 \\
\cline{2-5}
    & \multirow{9}{*}{N-pair}   & 0.1  & 88.65 ± 0.10  & 0.8870 ± 0.0016 \\
    &                          & 0.2  & 88.75 ± 0.09  & 0.8881 ± 0.0017 \\
    &                          & 0.25 & 88.85 ± 0.07  & 0.8883 ± 0.0010 \\
    &                          & 0.3  & 88.90 ± 0.08  & 0.8885 ± 0.0012 \\
    &                          & 0.4  & 88.95 ± 0.07  & 0.8890 ± 0.0010 \\
    &                          & 0.5  & 89.25 ± 0.09  & 0.8923 ± 0.0005 \\
    &                          & 0.6  & 89.00 ± 0.11  & 0.8895 ± 0.0010 \\
    &                          & 0.7  & 88.90 ± 0.12  & 0.8887 ± 0.0014 \\
    &                          & 0.75 & 88.71 ± 0.53  & 0.8869 ± 0.0044 \\
    &                          & 0.8  & 88.55 ± 0.52  & 0.8852 ± 0.0045 \\
    &                          & 0.9  & 88.45 ± 0.50  & 0.8840 ± 0.0040 \\
\cline{2-5}
    & \multirow{9}{*}{Magnet}  & 0.1  & 89.15 ± 0.28  & 0.8915 ± 0.0024 \\
    &                          & 0.2  & 89.22 ± 0.29  & 0.8919 ± 0.0026 \\
    &                          & 0.25 & 89.27 ± 0.29  & 0.8928 ± 0.0023 \\
    &                          & 0.3  & 89.35 ± 0.31  & 0.8933 ± 0.0025 \\
    &                          & 0.4  & 89.42 ± 0.33  & 0.8939 ± 0.0031 \\
    &                          & 0.5  & 89.07 ± 0.21  & 0.8911 ± 0.0022 \\
    &                          & 0.6  & 89.25 ± 0.33  & 0.8924 ± 0.0032 \\
    &                          & 0.7  & 89.45 ± 0.35  & 0.8939 ± 0.0035 \\
    &                          & 0.75 & \textbf{89.52 ± 0.34}  & \textbf{0.8946 ± 0.0040} \\
    &                          & 0.8  & 89.35 ± 0.32  & 0.8932 ± 0.0036 \\
    &                          & 0.9  & 89.30 ± 0.30  & 0.8925 ± 0.0034 \\
\hline
\end{tabular}
\end{table}

\begin{table}[ht]

\centering
\footnotesize
\caption{Baseline comparison with extended $\lambda$ values for CIFAR-10}
\label{tab:base_2}
\begin{tabular}{ccccc}

\textbf{Dataset} & \textbf{Loss Type} & $\boldsymbol{\lambda}$ & \textbf{Accuracy (Mean ± Std)} & \textbf{Micro-F1 (Mean ± Std)} \\
\hline
\multirow{45}{*}{\textbf{CIFAR-10}} 
    & Baseline & 0.0  & 85.88 ± 0.40  & 0.8586 ± 0.0042  \\
    \cline{2-5}
    & \multirow{9}{*}{Contrast}& 0.1  & 85.90 ± 0.95  & 0.8592 ± 0.0097 \\
    &                          & 0.2  & 85.95 ± 0.98  & 0.8596 ± 0.0099 \\
    &                          & 0.25 & 86.01 ± 0.99  & 0.8600 ± 0.0102 \\
    &                          & 0.3  & 86.10 ± 0.92  & 0.8608 ± 0.0095 \\
    &                          & 0.4  & 86.45 ± 0.70  & 0.8641 ± 0.0074 \\
    &                          & 0.5  & 86.87 ± 0.56  & 0.8693 ± 0.0049 \\
    &                          & 0.6  & 85.78 ± 0.48  & 0.8579 ± 0.0045 \\
    &                          & 0.7  & 85.30 ± 0.45  & 0.8523 ± 0.0041 \\
    &                          & 0.75 & 84.74 ± 0.44  & 0.8479 ± 0.0045 \\
    &                          & 0.8  & 84.12 ± 0.55  & 0.8418 ± 0.0052 \\
    &                          & 0.9  & 84.00 ± 0.52  & 0.8412 ± 0.0048 \\
\cline{2-5}
    & \multirow{9}{*}{Triplet} & 0.1  & 86.75 ± 0.27  & 0.8660 ± 0.0027 \\
    &                          & 0.2  & 86.78 ± 0.29  & 0.8662 ± 0.0029 \\
    &                          & 0.25 & 86.81 ± 0.25  & 0.8667 ± 0.0025 \\
    &                          & 0.3  & 86.85 ± 0.31  & 0.8670 ± 0.0028 \\
    &                          & 0.4  & 86.87 ± 0.37  & 0.8681 ± 0.0035 \\
    &                          & 0.5  & 86.88 ± 0.64  & 0.8683 ± 0.0059 \\
    &                          & 0.6  & 86.78 ± 0.52  & 0.8675 ± 0.0049 \\
    &                          & 0.7  & 86.70 ± 0.43  & 0.8665 ± 0.0037 \\
    &                          & 0.75 & 86.95 ± 0.42  & 0.8690 ± 0.0039 \\
    &                          & 0.8  & 86.70 ± 0.50  & 0.8669 ± 0.0053 \\
    &                          & 0.9  & 86.60 ± 0.38  & 0.8650 ± 0.0042 \\
\cline{2-5}
    & \multirow{9}{*}{N-pair}   & 0.1  & 84.80 ± 0.69  & 0.8463 ± 0.0065 \\
    &                          & 0.2  & 84.65 ± 0.72  & 0.8454 ± 0.0069 \\
    &                          & 0.25 & 84.52 ± 0.71  & 0.8446 ± 0.0067 \\
    &                          & 0.3  & 85.10 ± 0.63  & 0.8502 ± 0.0061 \\
    &                          & 0.4  & 85.70 ± 0.55  & 0.8561 ± 0.0052 \\
    &                          & 0.5  & 86.43 ± 0.78  & 0.8643 ± 0.0081 \\
    &                          & 0.6  & 85.63 ± 0.52  & 0.8563 ± 0.0057 \\
    &                          & 0.7  & 85.42 ± 0.47  & 0.8539 ± 0.0044 \\
    &                          & 0.75 & 85.91 ± 0.40  & 0.8583 ± 0.0042 \\
    &                          & 0.8  & 85.15 ± 0.45  & 0.8509 ± 0.0043 \\
    &                          & 0.9  & 85.23 ± 0.43  & 0.8521 ± 0.0045 \\
\cline{2-5}
    & \multirow{9}{*}{Magnet}  & 0.1  & 86.70 ± 0.65  & 0.8669 ± 0.0069 \\
    &                          & 0.2  & 86.85 ± 0.70  & 0.8683 ± 0.0072 \\
    &                          & 0.25 & 86.91 ± 0.69  & 0.8692 ± 0.0073 \\
    &                          & 0.3  & 87.10 ± 0.68  & 0.8702 ± 0.0071 \\
    &                          & 0.4  & 87.25 ± 0.85  & 0.8723 ± 0.0075 \\
    &                          & 0.5  & 86.72 ± 1.77  & 0.8671 ± 0.0174 \\
    &                          & 0.6  & 87.28 ± 0.79  & 0.8730 ± 0.0079 \\
    &                          & 0.7  & 87.20 ± 0.88  & 0.8719 ± 0.0084 \\
    &                          & 0.75 & \textbf{87.36 ± 0.82}  & \textbf{0.8738 ± 0.0081} \\
    &                          & 0.8  & 87.05 ± 0.70  & 0.8708 ± 0.0076 \\
    &                          & 0.9  & 87.10 ± 0.59  & 0.8714 ± 0.0056 \\
    \hline
\end{tabular}
\end{table}

\begin{table}[!ht]
\centering
\footnotesize
\caption{Baseline comparison with extended $\lambda$ values for CIFAR-100}
\label{tab:base_3}
\begin{tabular}{ccccc}

\textbf{Dataset} & \textbf{Loss Type} & $\boldsymbol{\lambda}$ & \textbf{Accuracy (Mean ± Std)} & \textbf{Micro-F1 (Mean ± Std)} \\
\hline
\multirow{45}{*}{\textbf{CIFAR-100}} 
    & Baseline & 0.0  & 61.77 ± 0.49  & 0.6163 ± 0.0064 \\
    \cline{2-5}
    & \multirow{9}{*}{Contrast}& 0.1  & 61.05 ± 0.83  & 0.6088 ± 0.0071 \\
    &                          & 0.2  & 61.25 ± 0.75  & 0.6102 ± 0.0079 \\
    &                          & 0.25 & 61.04 ± 0.81  & 0.6088 ± 0.0087 \\
    &                          & 0.3  & 60.85 ± 0.80  & 0.6067 ± 0.0082 \\
    &                          & 0.4  & 60.50 ± 0.78  & 0.6045 ± 0.0079 \\
    &                          & 0.5  & 60.30 ± 0.79  & 0.6021 ± 0.0078 \\
    &                          & 0.6  & 60.10 ± 0.85  & 0.6004 ± 0.0079 \\
    &                          & 0.7  & 59.90 ± 0.84  & 0.5985 ± 0.0078 \\
    &                          & 0.75 & 59.88 ± 0.85  & 0.5982 ± 0.0082 \\
    &                          & 0.8  & 59.70 ± 0.80  & 0.5965 ± 0.0081 \\
    &                          & 0.9  & 59.50 ± 0.85  & 0.5948 ± 0.0085 \\
\cline{2-5}
    & \multirow{9}{*}{Triplet} & 0.1  & 62.10 ± 0.75  & 0.6202 ± 0.0074 \\
    &                          & 0.2  & 62.30 ± 0.70  & 0.6215 ± 0.0075 \\
    &                          & 0.25 & 62.50 ± 0.70  & 0.6228 ± 0.0075 \\
    &                          & 0.3  & 62.55 ± 0.72  & 0.6230 ± 0.0076 \\
    &                          & 0.4  & 62.60 ± 0.70  & 0.6235 ± 0.0073 \\
    &                          & 0.5  & 62.75 ± 0.68  & 0.6240 ± 0.0071 \\
    &                          & 0.6  & 62.80 ± 0.69  & 0.6245 ± 0.0072 \\
    &                          & 0.7  & 62.65 ± 0.70  & 0.6237 ± 0.0073 \\
    &                          & 0.75 & 62.70 ± 0.72  & 0.6240 ± 0.0075 \\
    &                          & 0.8  & 62.40 ± 0.70  & 0.6215 ± 0.0073 \\
    &                          & 0.9  & 62.30 ± 0.68  & 0.6212 ± 0.0071 \\
\cline{2-5}
    & \multirow{9}{*}{N-pair}   & 0.1  & 61.20 ± 0.75  & 0.6104 ± 0.0076 \\
    &                          & 0.2  & 61.25 ± 0.70  & 0.6110 ± 0.0074 \\
    &                          & 0.25 & 61.30 ± 0.75  & 0.6115 ± 0.0075 \\
    &                          & 0.3  & 61.35 ± 0.70  & 0.6118 ± 0.0073 \\
    &                          & 0.4  & 61.40 ± 0.80  & 0.6121 ± 0.0074 \\
    &                          & 0.5  & 61.50 ± 0.75  & 0.6130 ± 0.0076 \\
    &                          & 0.6  & 61.60 ± 0.70  & 0.6135 ± 0.0073 \\
    &                          & 0.7  & 61.55 ± 0.80  & 0.6130 ± 0.0079 \\
    &                          & 0.75 & 61.60 ± 0.70  & 0.6135 ± 0.0074 \\
    &                          & 0.8  & 61.55 ± 0.72  & 0.6132 ± 0.0075 \\
    &                          & 0.9  & 61.50 ± 0.68  & 0.6129 ± 0.0071 \\
\cline{2-5}
    & \multirow{9}{*}{Magnet}  & 0.1  & 62.80 ± 0.69  & 0.6242 ± 0.0072 \\
    &                          & 0.2  & 63.00 ± 0.75  & 0.6250 ± 0.0076 \\
    &                          & 0.25 & 63.20 ± 0.70  & 0.6265 ± 0.0075 \\
    &                          & 0.3  & 63.25 ± 0.70  & 0.6267 ± 0.0074 \\
    &                          & 0.4  & 63.30 ± 0.75  & 0.6270 ± 0.0076 \\
    &                          & 0.5  & 63.40 ± 0.70  & 0.6275 ± 0.0075 \\
    &                          & 0.6  & 63.45 ± 0.75  & 0.6277 ± 0.0076 \\
    &                          & 0.7  & 63.30 ± 0.72  & 0.6268 ± 0.0075 \\
    &                          & 0.75 & \textbf{63.50 ± 0.70}  & \textbf{0.6285 ± 0.0072} \\
    &                          & 0.8  & 63.35 ± 0.72  & 0.6273 ± 0.0076 \\
    &                          & 0.9  & 63.30 ± 0.68  & 0.6270 ± 0.0071 \\
\hline
\end{tabular}
\end{table}

% \section{Latent Boost Hyperparameter}
% \label{app:latent_boost}
% As an addition to the introduced scheduling of $\alpha$ and $\beta$ within our \name{} approach as introduced in \Cref{sec:latentboost}, we present an exemplary schedule of hyperparameters across 100 epochs in \Cref{fig:simulate}.
% Throughout our experiments, we initialized and dynamically changed the two hyperparameters according to that process.

% \begin{figure}[ht]
%     \centering
%     \includegraphics[width=0.6\textwidth]{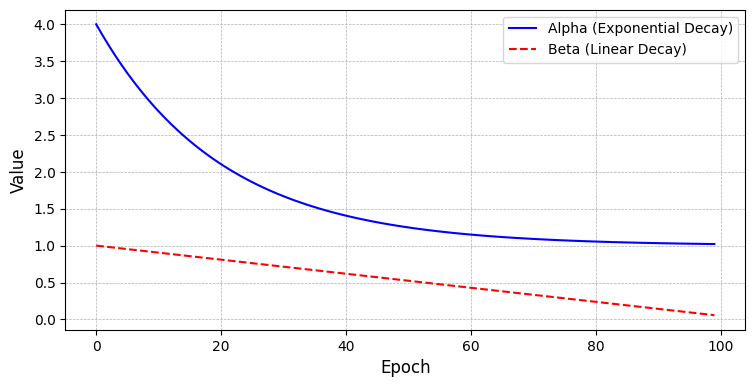}
%     \caption{Example based on 100 epochs for the exponential decrease of $\alpha$ and linear decrease of $\beta$ to dynamically adapt the importance of intra- and inter-class loss between cluster in the \name{} approach.}
%     \label{fig:simulate}
% \end{figure}
